# Supplementary material for: Audio-Visual Scene-Aware Dialog
Source: arXiv:1901.09107 source file (2019-05-08)
Supplement: Supplementary file 1 [file section_AVSD_interface.tex]

%%%%%%%%%%%%%%%%%%%%%%%%%%%%%%%%%%%%%%%%%%%%%%%%%%%%%%%%%%%

\vspace{\sectionReduceTop}
\section{Interface.}
\vspace{\sectionReduceBot}
\label{sec:section_interface}
TODO
